# Supplementary material for: Automatic Mixed-Precision Quantization Search of BERT
Source: arXiv:2112.14938 source file (2021-12-30)
Supplement: Supplementary file 1 [file appendix.tex]

\begin{figure*}[t!]
\caption{Evolution of the validation loss and model size over the course of training on the SST-2 dataset. The desirable model size is 30M.  }
\label{fig:loss_evl}
  \begin{minipage}{0.48\textwidth}
\includegraphics[width=\columnwidth]{./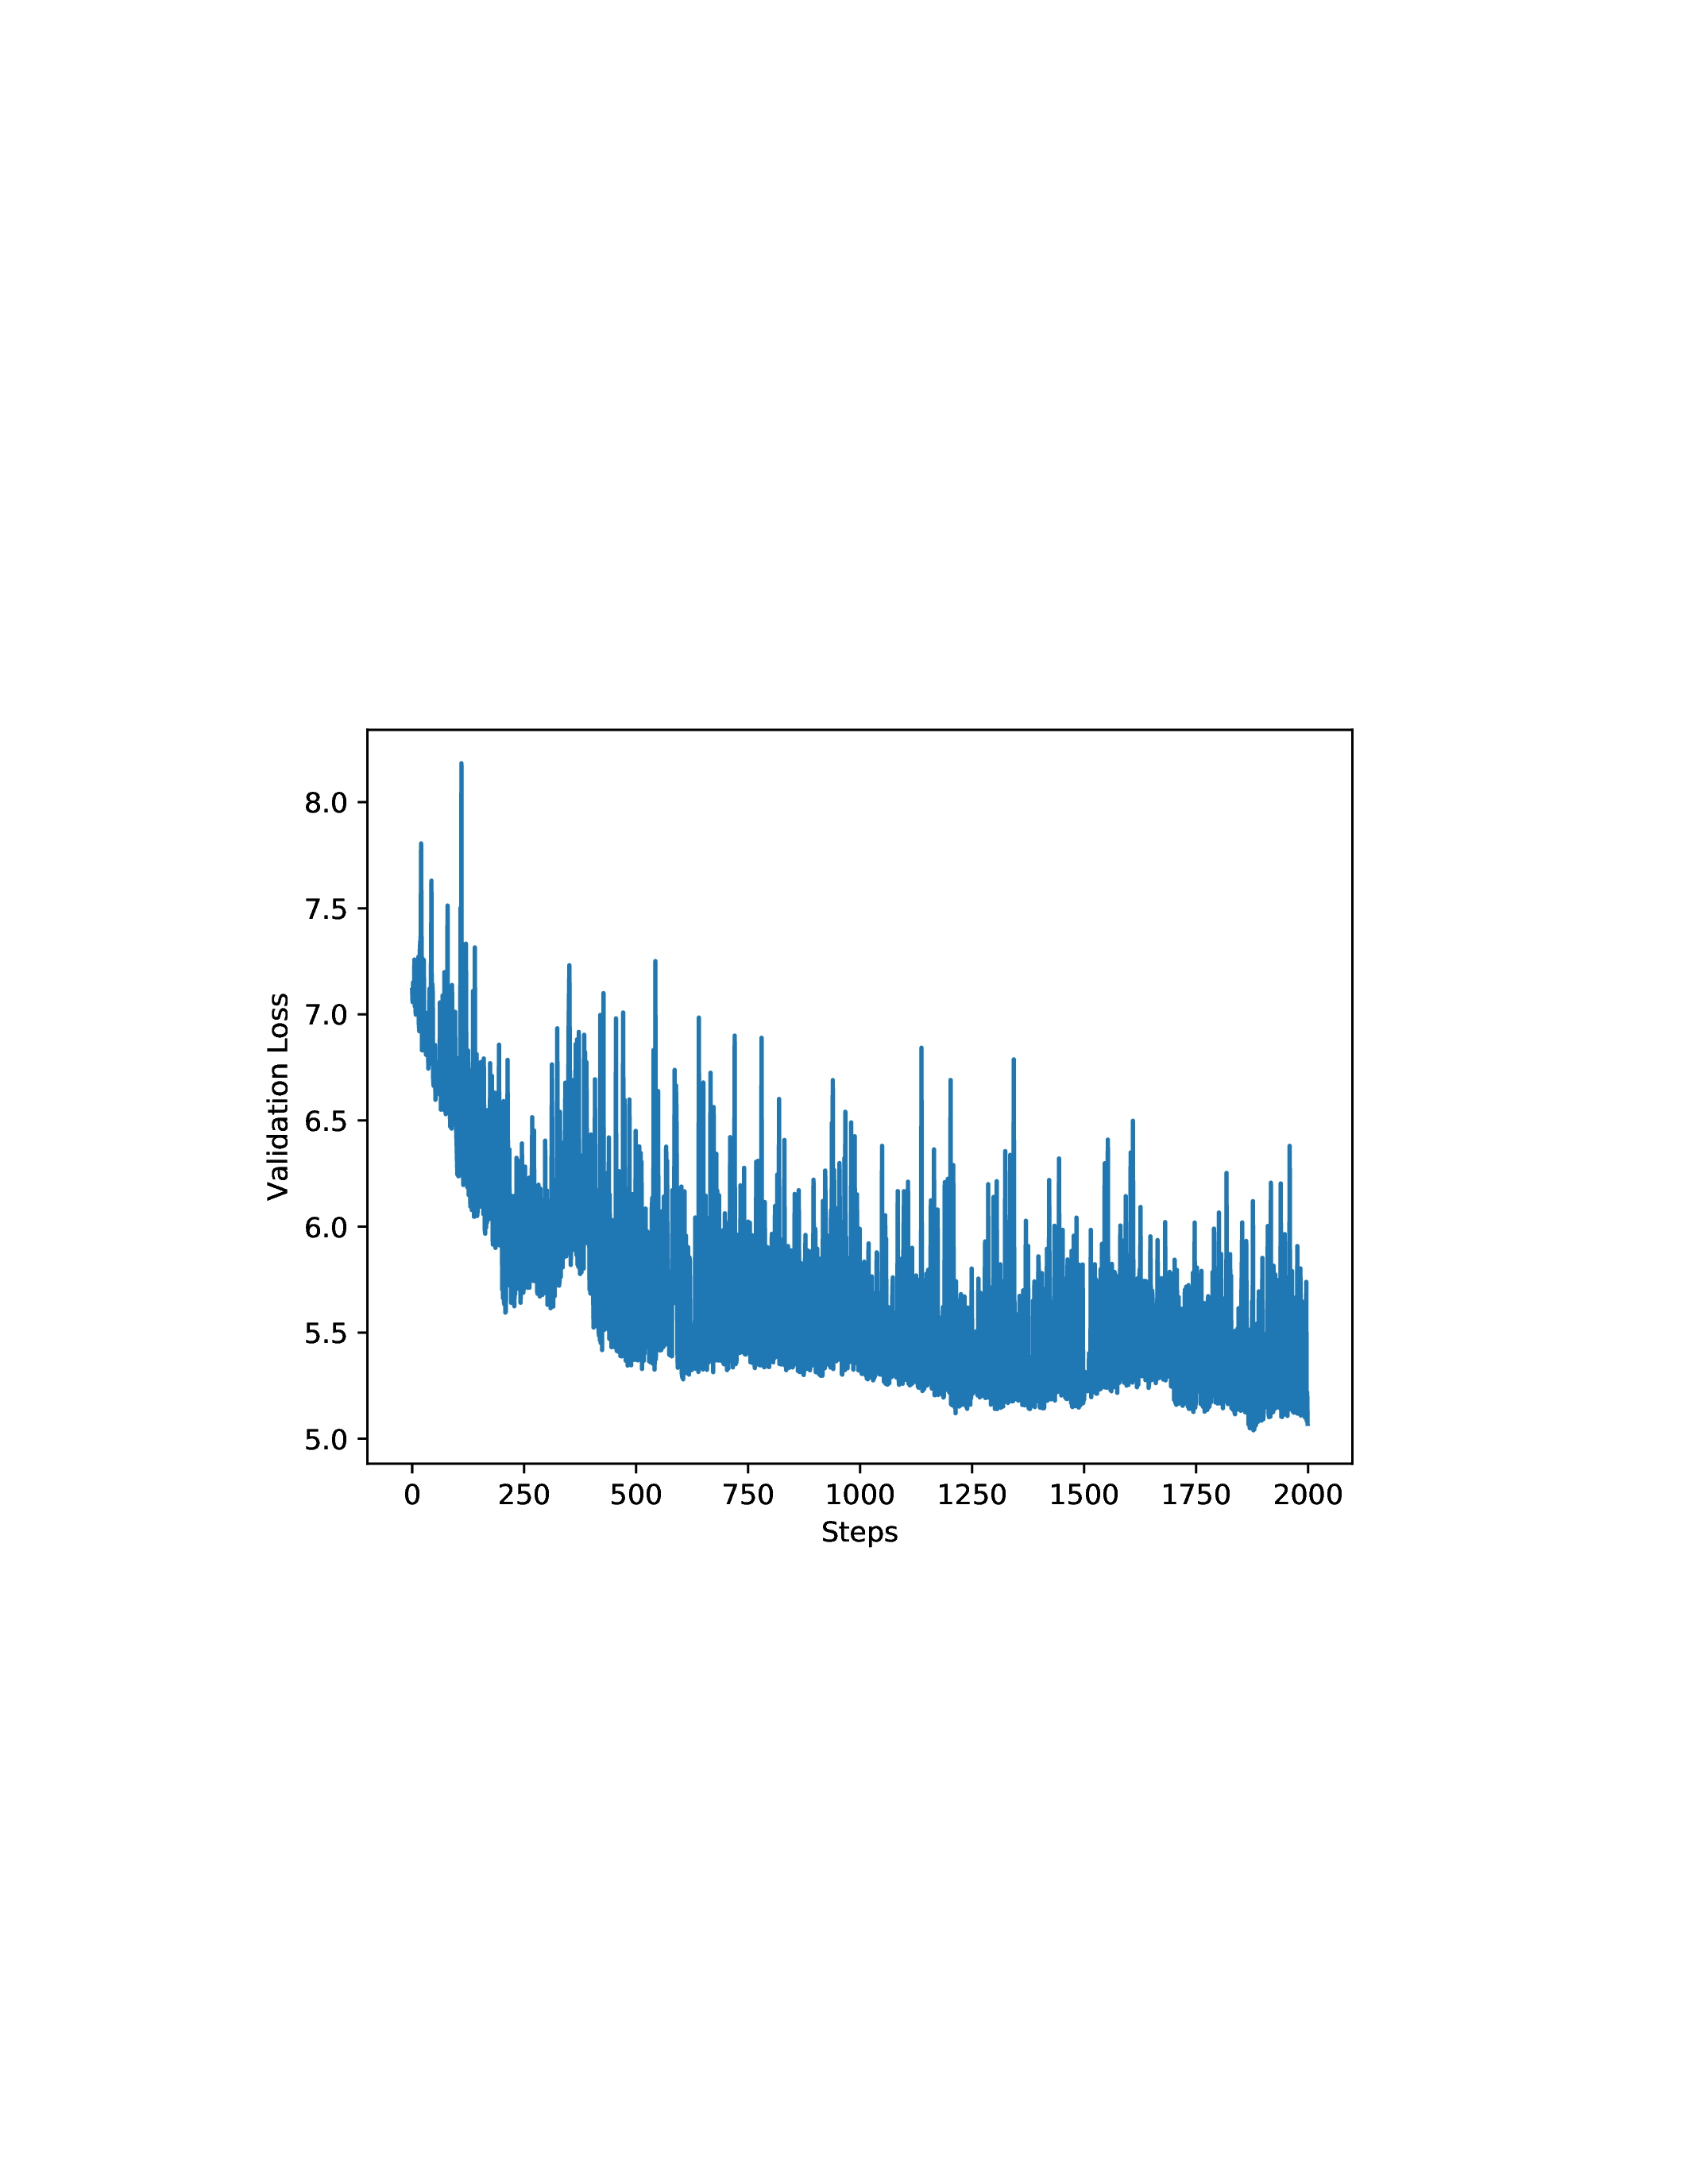}
\subcaption{Validation Loss  $\mathcal{L}_{\rm{val}}$ }
\label{fig:Exemplar_73}
\end{minipage}
  \begin{minipage}{0.48\textwidth}
\includegraphics[width=\columnwidth]{./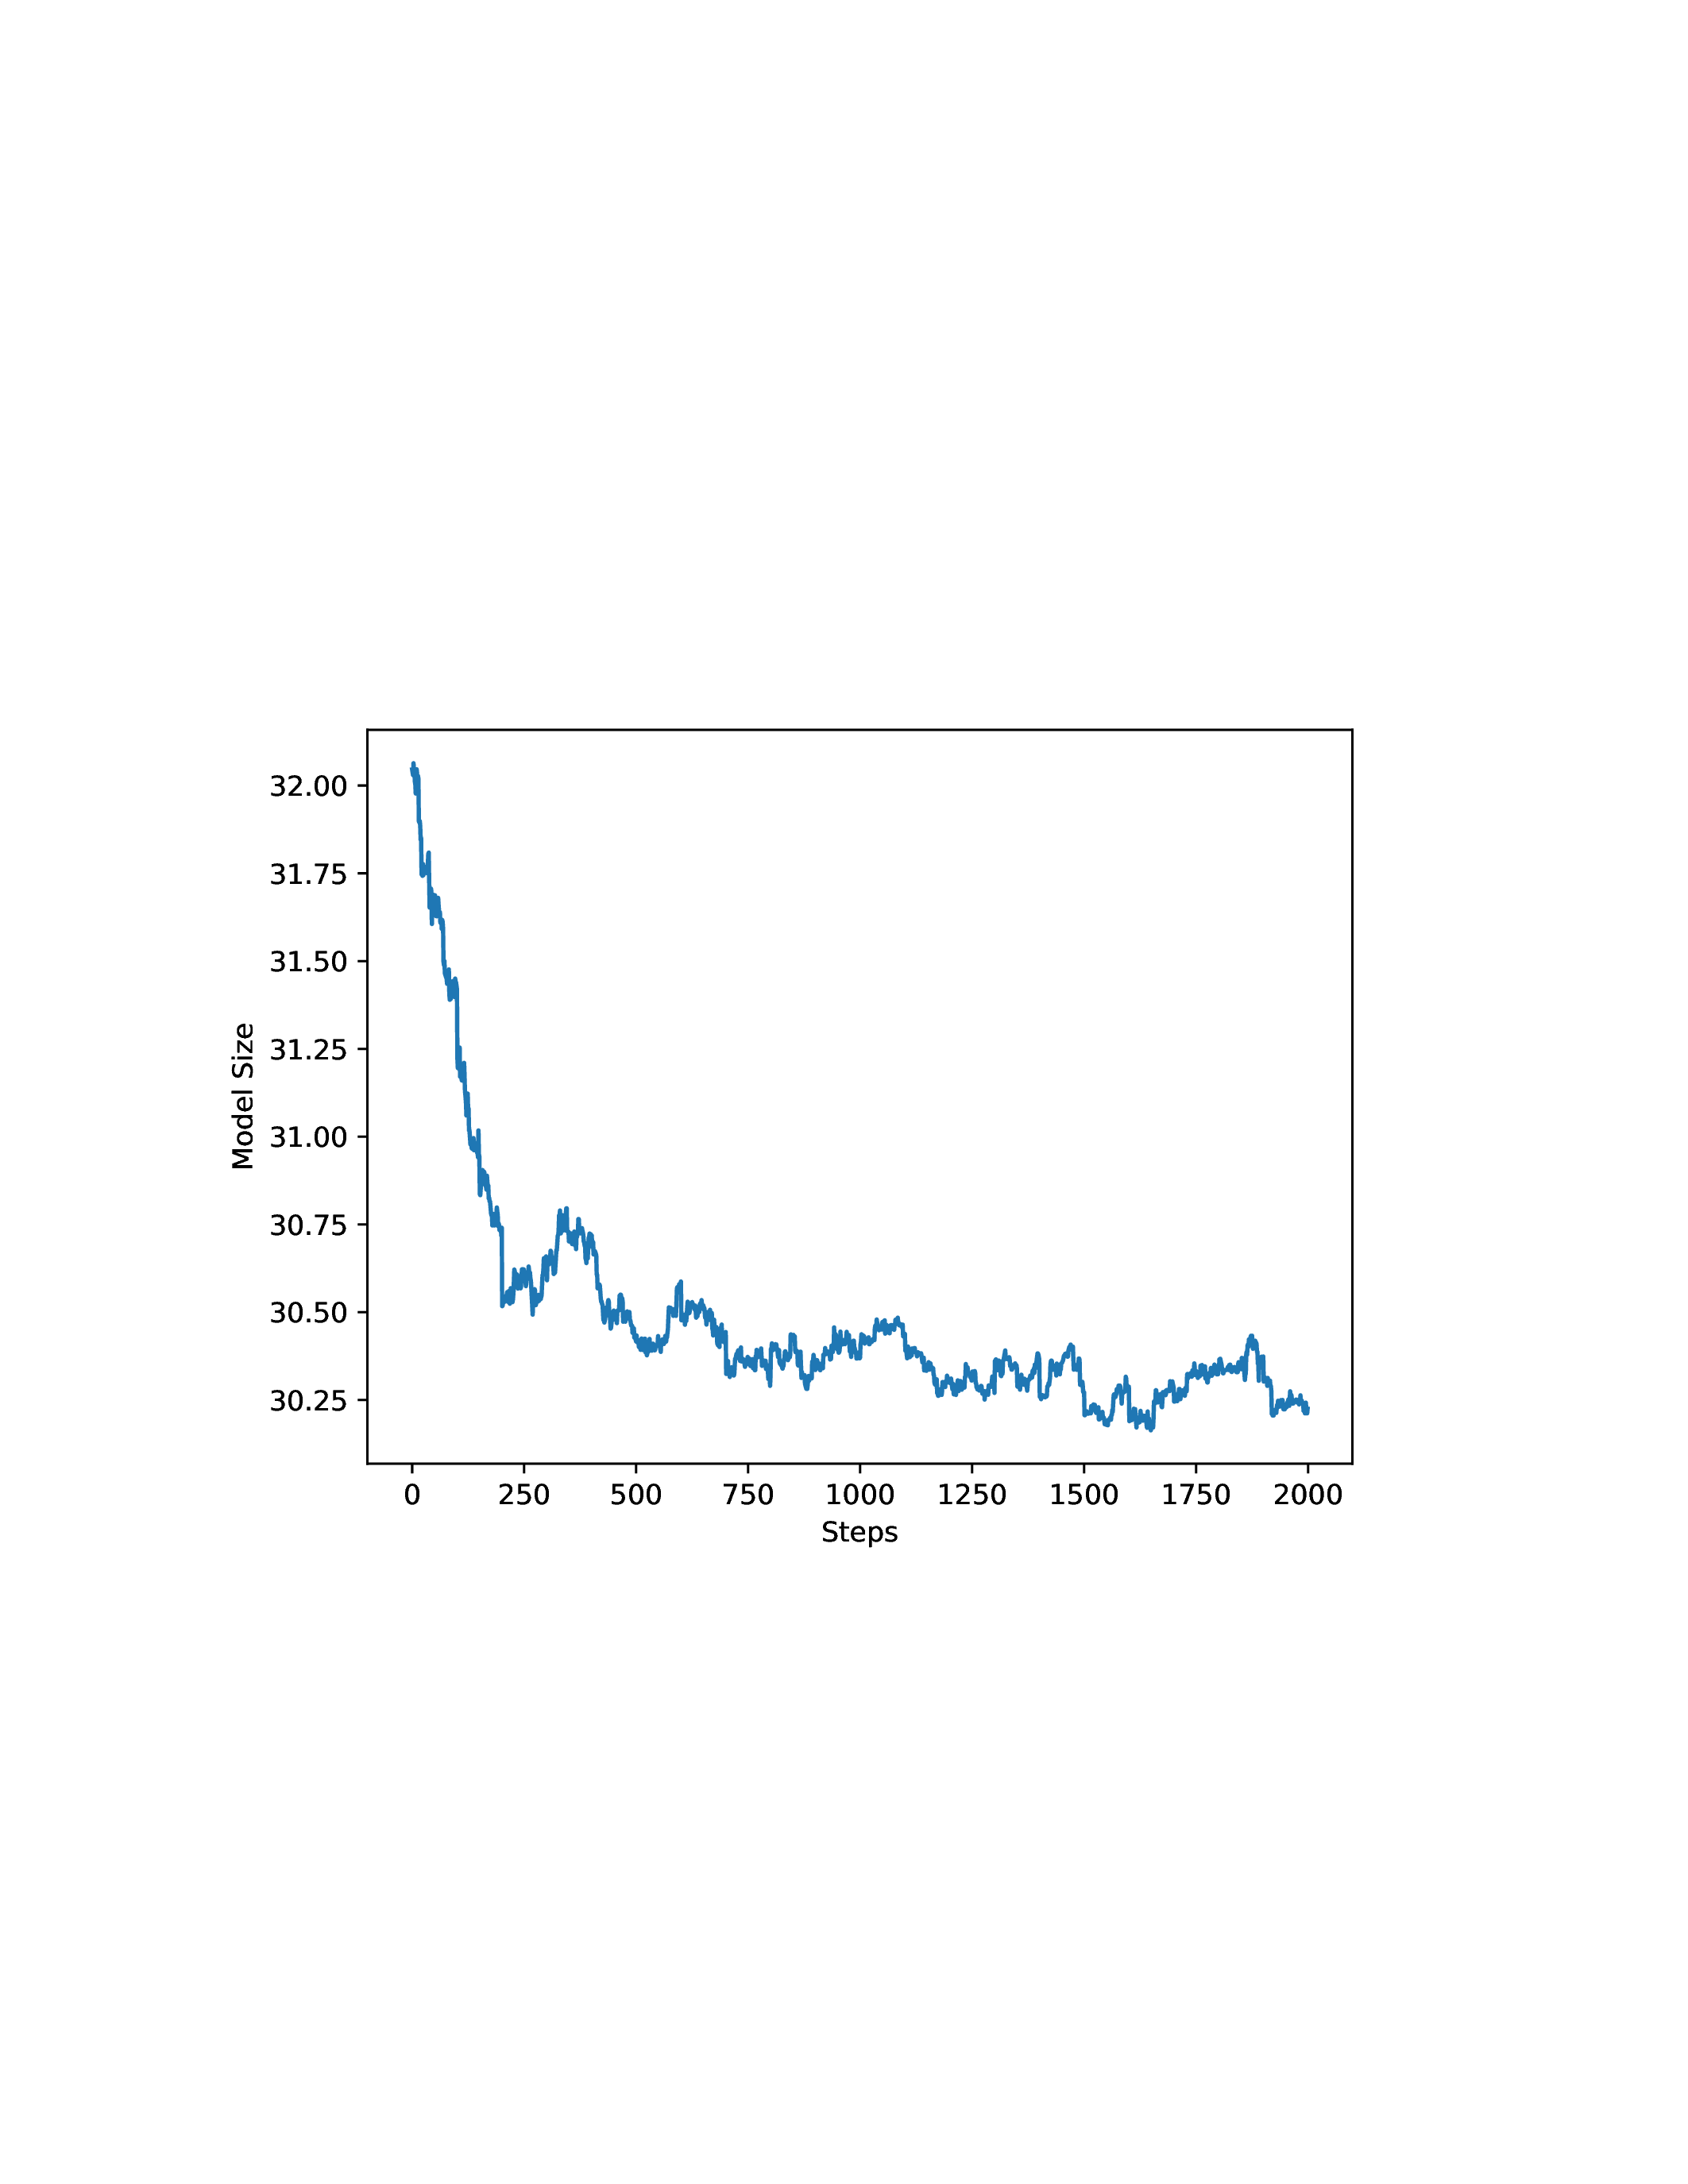}
\subcaption{Model Size $C_{\mathcal{O}}$}
\label{fig:Exemplar_150}
\end{minipage}
\end{figure*}

\section{Experimental Setup Details}
\label{sec:app_exp_details}
In this part, we describe the implementation details of the baselines and our proposed AQ-BERT.
\subsection{BERT-base and Distilbert model}
Our implementation is based on transformers by huggingface\footnote{https://github.com/huggingface/transformers}.
The default hyperparameters settings are used for training bert-base and Distilbert-base models. 
Specifically, the original bert-base model contains 109M parameters: the number of layers is 12, the hidden size is 768,  the feed-forward/filter size is 3072, and the head number is 12. 

\subsubsection{\kmethod} 
Our method contains multiple processes: quantization, continuous relaxation, and optimization. 
In this part, we first describe the setting for each module respectively, and then introduce the overall process and validation details. 
\begin{itemize}
    \item \textbf{Quantization}.
    Our weight quantization follows the implementation of \cite{zhang2020precision}, with embedding layer and activation quantized to 8 bit. We conduct the architecture search at each subgroup.  To examine our model capability in extreme low bit mixed-precision quantization, we only choose precision from  {0,1,2,3,4}. We calculate scale and zero points for each subgroup every 100 steps during quant-aware training for a good balance of accuracy and speed. Dedicated hardware support is needed to fully utilize the speedup and save the memory of quantization during inference.
    
\item \textbf{Continuous Relaxation}. The initial temperature for Softmax function is set to 1 and decay rate $\eta=4$ per epoch in Equation \ref{equ:temp}, with each task normally converges in 5 epochs.

\item \textbf{Optimization}. Both inner network and super network are trained with batch size of 32.
We use AdamW optimizer with a learning rate of $2e-5$ and $\epsilon$ of $1e-8$, and set SGD with a learning rate of 0.1 for architecture optimization.

\item \textbf{Overall process}.
To prepare the weights for ultra-low precision quantization, the model is first trained without architecture search in 8 bit for 1000  warm-up steps. 
After that, the architecture training is gradually unfrozen. 
Specifically, for every 1000 steps, the bit assignments are randomly initialized layer by layer. 
For the unfrozen architecture, we first conduct 100 training steps, followed by 100 architecture updates. 
\item \textbf{Validation}.
We randomly split the training set into two parts.  
90\% of the data is used to train the model weights, and left 10\% data are served as the validation set for the training of the architecture parameters. 
After the training, we initialize the model with searched architecture and train from scratch with the whole training split. We evaluate model accuracy on a standard test set.
\end{itemize}

\section{Convergence}
Figure \ref{fig:loss_evl} shows the evolution of validation loss  $\mathcal{L}_{\rm{val}}$ calculated via Equation \ref{equ:loss_val} and model size $C_{\mathcal{O}}$ calculated via  Equation \ref{equ:C_o} on SST-2 dataset, when the desirable model size is $30M$.
Although our method is not the same as the standard optimization process that converges when the gradient is zero, our approach can reach a fixed stage in practice.
As can be seen from Figure \ref{fig:loss_evl}, within 2,000 steps, model size $C_{\mathcal{O}}$ fast converges to the desirable size $30$M, and validation loss $\mathcal{L}_{\rm{val}}$ reaches to a comparatively fixed value. 
These phenomenons show that our faster inference is sufficient in practical usage.
